# Supplementary material for: Properties of spherical and deformed nuclei using regularized pseudopotentials in nuclear DFT
Source: arXiv:2003.10990 source file (2020-03-28)
Supplement: Supplementary file 1 [file RegPseudoPot-supp-05.pdf]

# Supplemental material for: Properties of spherical and deformed nuclei using regularized pseudopotentials in nuclear DFT

**K Bennaceur[1], J Dobaczewski[2,3,4], T Haverinen[4,5], and M Kortelainen[5,4]**

[1]Univ Lyon, Université Claude Bernard Lyon 1, CNRS, IPNL, UMR 5822, 4 rue E. Fermi, F-69622 Villeurbanne Cedex, France
[2]Department of Physics, University of York, Heslington, York YO10 5DD, United Kingdom
[3]Institute of Theoretical Physics, Faculty of Physics, University of Warsaw, Pasteura 5, 02-093 Warszawa, Poland
[4]Helsinki Institute of Physics, P.O. Box 64, 00014 University of Helsinki, Finland
[5]Department of Physics, University of Jyväskylä, P.O. Box 35 (YFL), 40014 University of Jyväskylä, Finland

Submitted to: *J. Phys. G: Nucl. Phys.*

## 6. Numerical parameters

Numerical calculations presented in this study were performed by employing codes FINRES$_4$ [1] (spherical symmetry in the coordinate representation), HFBTEMP [2] (axial symmetry in the harmonic-oscillator basis), and HFODD (v2.92a) [3, 4] (3D symmetry in the harmonic-oscillator basis). Values of the two essential physical constants, which determine the self-consistent solutions, were the nucleon mass, amounting to $\hbar^2/2m = 20.736676229\,\mathrm{MeV\,fm}^2$, and elementary charge squared of $e^2 = 1.4399784086\,\mathrm{MeV\,fm}$. The two-body center-of-mass correction and exact Coulomb-exchange term were included [5], whereas the Coulomb-force and spin-orbit contributions to the pairing channel were neglected.

## 7. Parameters of pseudopotentials and covariance matrices

Parameters of the pseudopotentials adjusted in this study in steps 2 and 3, see Sec. 3, are listed in files `Parameters.step2.txt` and `Parameters.step3.txt`, respectively. In both files, each line gives the effective mass, $m^*/m$, order of the pseudopotential $n$, range $a$ (in fm), and the parameters ordered as: $t_3$ (in $\mathrm{MeV\,fm}^4$), $W_{\mathrm{SO}}$ (in $\mathrm{MeV\,fm}^5$), $W_1^{(0)}$, $B_1^{(0)}$, $H_1^{(0)}$, $M_1^{(0)}$, $W_1^{(2)}$, $B_1^{(2)}$, $H_1^{(2)}$, $M_1^{(2)}$, $W_1^{(4)}$, $B_1^{(4)}$, $H_1^{(4)}$, $M_1^{(4)}$, $W_1^{(6)}$, $B_1^{(6)}$, $H_1^{(6)}$, and $M_1^{(6)}$ (in $\mathrm{MeV\,fm}^{3+n}$.

Parameter sets listed in file `Parameters.step2.txt` are not given any names, whereas those in `Parameters.step2.txt` are named as REG$n$m.190617, see Sec. 3.

Covariance matrices that correspond to pseudopotentials REG6a.190617 and REG6d.190617 are listed in files `Covariance.matrix.REG6a.190617.txt` and `Covariance.matrix.REG6d.190617.txt`, respectively. Both covariance matrices were evaluated with 11 eigenvectors of the Hessian matrices kept. The order of parameters is the same as that for the files with parameters described above.

This work was partially supported by the STFC Grants No. ST/M006433/1 and No. ST/P003885/1, and by the Polish National Science Centre under Contract No. 2018/31/B/ST2/02220. We acknowledge the CSC-IT Center for Science Ltd. (Finland) and the IN2P3 Computing Center (CNRS, Lyon-Villeurbanne, France) for the allocation of computational resources.

## References

[1] Bennaceur K *et al.*, unpublished

[2] Kortelainen M *et al.*, unpublished

[3] Schunck N, Dobaczewski J, Satuła W, Bączyk P, Dudek J, Gao Y, Konieczka M, Sato K, Shi Y, Wang X and Werner T 2017 *Comp. Phys. Commun.* **216** 145 – 174 URL `http://www.sciencedirect.com/science/article/pii/S0010465517300942`

[4] Dobaczewski J 2020 *et al.*, to be published

[5] Bender M, Heenen P H and Reinhard P G 2003 *Rev. Mod. Phys.* **75**(1) 121–180 URL `https://link.aps.org/doi/10.1103/RevModPhys.75.121`
